# Supplementary material for: On the group-theoretic structure of lifted filter banks
Source: arXiv:1310.0530 ancillary file (2014-09-25)
Supplement: Supplementary file 1 [file Brislawn_AMS_ABQ_2014_slides.pdf]

# Groups of Linear Phase Filter Banks

Christopher M. Brislawn

Group CCS-3, Information Sciences  
Computer, Computational, and Statistical Sciences Division  
Los Alamos National Laboratory, Los Alamos, NM

<http://www.ccs3.lanl.gov/group/people/?id=brislawn>

<http://www.linkedin.com/profile/view?id=19087822>  
brislawn@lanl.gov

AMS Special Session on Harmonic Analysis and Applications  
University of New Mexico, 5 April 2014

Research supported by LANL Laboratory-Directed R&D Funding, Kristi D. and Reilly R. Brislawn.

LA-UR-12-21217

# Outline [1]

- 1 Two-Channel FIR Perfect Reconstruction Filter Banks
- 2 How Unique Are Lifting Factorizations?
- 3 Unique Group Lifting Factorization Theorem
- 4 Group Theoretic Structure
- 5 Work In Progress
- 6 References

# Two-Channel FIR Perfect Reconstruction Filter Banks

- Direct-form Z-transform representation of a discrete-time filter bank:

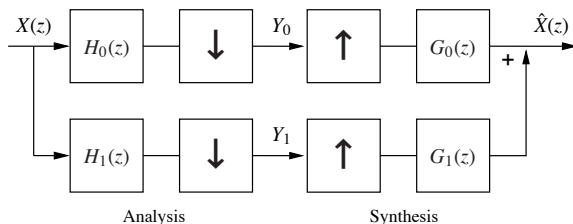

# Two-Channel FIR Perfect Reconstruction Filter Banks

- Direct-form Z-transform representation of a discrete-time filter bank:

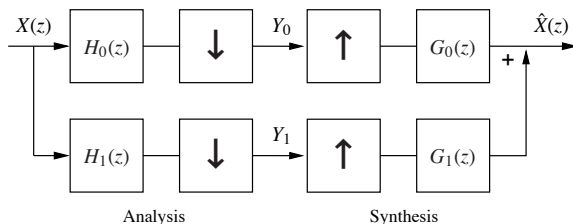

- This is equivalent to a *polyphase transfer matrix representation*,  $\mathbf{Y}(z) = \mathbf{H}(z) \mathbf{X}(z)$ :

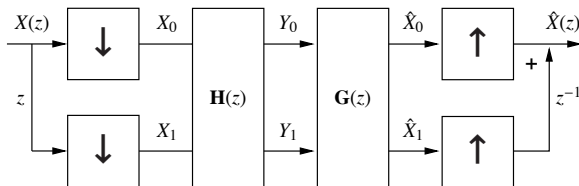

# Lifting Factorization of Polyphase Matrices

- Assume  $\mathbf{H}(z)$  is in the *unimodular group*,  $|\mathbf{H}(z)| = 1$ , and factor  $\mathbf{H}(z)$  into elementary matrices over  $\mathbb{C}[z, z^{-1}]$ , e.g.:

$$\mathbf{H}(z) = \mathbf{D}_K \mathbf{S}_1(z) \mathbf{S}_0(z), \quad \mathbf{D}_K \equiv \text{diag}(1/K, K),$$

$$\mathbf{S}_0(z) = \begin{bmatrix} 1 & S_0(z) \\ 0 & 1 \end{bmatrix}, \quad \mathbf{S}_1(z) = \begin{bmatrix} 1 & 0 \\ S_1(z) & 1 \end{bmatrix}$$

# Lifting Factorization of Polyphase Matrices

- Assume  $\mathbf{H}(z)$  is in the *unimodular group*,  $|\mathbf{H}(z)| = 1$ , and factor  $\mathbf{H}(z)$  into elementary matrices over  $\mathbb{C}[z, z^{-1}]$ , e.g.:

$$\mathbf{H}(z) = \mathbf{D}_K \mathbf{S}_1(z) \mathbf{S}_0(z), \quad \mathbf{D}_K \equiv \text{diag}(1/K, K),$$

$$\mathbf{S}_0(z) = \begin{bmatrix} 1 & S_0(z) \\ 0 & 1 \end{bmatrix}, \quad \mathbf{S}_1(z) = \begin{bmatrix} 1 & 0 \\ S_1(z) & 1 \end{bmatrix}$$

- Lifting updates one channel w. filtered version of other channel:

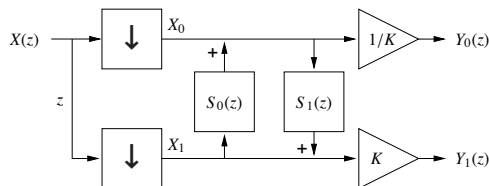

# Lifting Factorization of Polyphase Matrices

- Assume  $\mathbf{H}(z)$  is in the *unimodular group*,  $|\mathbf{H}(z)| = 1$ , and factor  $\mathbf{H}(z)$  into elementary matrices over  $\mathbb{C}[z, z^{-1}]$ , e.g.:

$$\mathbf{H}(z) = \mathbf{D}_K \mathbf{S}_1(z) \mathbf{S}_0(z), \quad \mathbf{D}_K \equiv \text{diag}(1/K, K),$$

$$\mathbf{S}_0(z) = \begin{bmatrix} 1 & S_0(z) \\ 0 & 1 \end{bmatrix}, \quad \mathbf{S}_1(z) = \begin{bmatrix} 1 & 0 \\ S_1(z) & 1 \end{bmatrix}$$

- Lifting updates one channel w. filtered version of other channel:

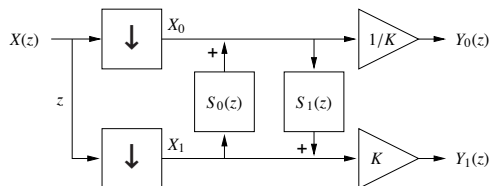

- Daubechies & Sweldens proved that all unimodular FIR filter banks factor this way.

# Linear Phase FIR Biorthogonal Filter Banks

- Two classes, corresponding to symmetric (antisym.) wavelets:

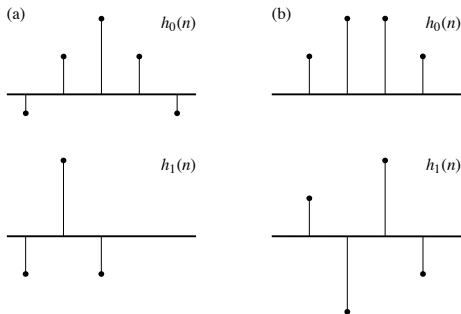

(a) whole-sample symmetric (WS), (b) half-sample symmetric (HS)

# Linear Phase FIR Biorthogonal Filter Banks

- Two classes, corresponding to symmetric (antisym.) wavelets:

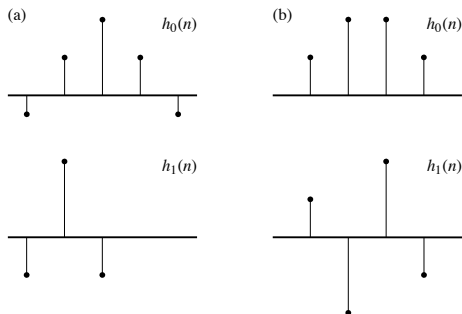

(a) whole-sample symmetric (WS), (b) half-sample symmetric (HS)

- An analysis bank is WS (about 0 and  $-1$ ) iff

$$\mathbf{H}(z^{-1}) = \mathbf{\Lambda}(z) \mathbf{H}(z) \mathbf{\Lambda}(z^{-1}) \quad \text{where} \quad \mathbf{\Lambda}(z) \equiv \text{diag}(1, z^{-1}) .$$

Let  $\mathcal{W}$  be the group of all unimodular WS polyphase matrices.

# Lifting Factorization of WS Filter Banks in $\mathcal{W}$ [2]

- A lifting matrix  $\mathbf{S}(z)$  is in  $\mathcal{W}$  iff its lifting filter  $S(z)$  is HS, where:
  - 1  $S(z)$  is symmetric about  $1/2$  if  $\mathbf{S}(z)$  is upper-triangular, or
  - 2  $S(z)$  is symmetric about  $-1/2$  if  $\mathbf{S}(z)$  is lower-triangular.

The *upper-triangular WS lifting group*,  $\mathcal{U}$ , is the group of lifting matrices satisfying (1). The *lower-triangular WS lifting group*,  $\mathcal{L}$ , is the group satisfying (2).

# Lifting Factorization of WS Filter Banks in $\mathcal{W}$ [2]

- A lifting matrix  $\mathbf{S}(z)$  is in  $\mathcal{W}$  iff its lifting filter  $S(z)$  is HS, where:
  - ①  $S(z)$  is symmetric about  $1/2$  if  $\mathbf{S}(z)$  is upper-triangular, or
  - ②  $S(z)$  is symmetric about  $-1/2$  if  $\mathbf{S}(z)$  is lower-triangular.

The *upper-triangular WS lifting group*,  $\mathcal{U}$ , is the group of lifting matrices satisfying (1). The *lower-triangular WS lifting group*,  $\mathcal{L}$ , is the group satisfying (2).

- **Theorem:** (WS Lifting Factorization)  $\mathbf{H}(z) \in \mathcal{W}$  iff it factors as

$$\mathbf{H}(z) = \mathbf{D}_K \mathbf{S}_N(z) \cdots \mathbf{S}_0(z), \quad \mathbf{D}_K \equiv \text{diag}(1/K, K), \quad \mathbf{S}_i \in \mathcal{U} \cup \mathcal{L}.$$

# Lifting Factorization of WS Filter Banks in $\mathcal{W}$ [2]

- A lifting matrix  $\mathbf{S}(z)$  is in  $\mathcal{W}$  iff its lifting filter  $S(z)$  is HS, where:

- ①  $S(z)$  is symmetric about  $1/2$  if  $\mathbf{S}(z)$  is upper-triangular, or
- ②  $S(z)$  is symmetric about  $-1/2$  if  $\mathbf{S}(z)$  is lower-triangular.

The *upper-triangular WS lifting group*,  $\mathcal{U}$ , is the group of lifting matrices satisfying (1). The *lower-triangular WS lifting group*,  $\mathcal{L}$ , is the group satisfying (2).

- **Theorem:** (WS Lifting Factorization)  $\mathbf{H}(z) \in \mathcal{W}$  iff it factors as

$$\mathbf{H}(z) = \mathbf{D}_K \mathbf{S}_N(z) \cdots \mathbf{S}_0(z), \quad \mathbf{D}_K \equiv \text{diag}(1/K, K), \quad \mathbf{S}_i \in \mathcal{U} \cup \mathcal{L}.$$

- Define the *gain scaling group*,  $\mathcal{D} \equiv \{\mathbf{D}_K : K \neq 0\}$ .

The *lifting cascade group* is  $\mathcal{C} \equiv \langle \mathcal{U} \cup \mathcal{L} \rangle < \mathcal{W}$ .

$\mathcal{D}$  acts on  $\mathcal{U}$ ,  $\mathcal{L}$ ,  $\mathcal{C}$  via inner automorphisms,  $\gamma_K \mathbf{A}(z) \equiv \mathbf{D}_K \mathbf{A}(z) \mathbf{D}_K^{-1}$ .

We say “ $\mathcal{D}$  normalizes  $\mathcal{C}$ ,” or “ $\mathcal{C}$  is  $\mathcal{D}$ -invariant.”

# Lifting Factorization of WS Filter Banks in $\mathcal{W}$ [2]

- A lifting matrix  $\mathbf{S}(z)$  is in  $\mathcal{W}$  iff its lifting filter  $S(z)$  is HS, where:

- ①  $S(z)$  is symmetric about  $1/2$  if  $\mathbf{S}(z)$  is upper-triangular, or
- ②  $S(z)$  is symmetric about  $-1/2$  if  $\mathbf{S}(z)$  is lower-triangular.

The *upper-triangular WS lifting group*,  $\mathcal{U}$ , is the group of lifting matrices satisfying (1). The *lower-triangular WS lifting group*,  $\mathcal{L}$ , is the group satisfying (2).

- **Theorem:** (WS Lifting Factorization)  $\mathbf{H}(z) \in \mathcal{W}$  iff it factors as

$$\mathbf{H}(z) = \mathbf{D}_K \mathbf{S}_N(z) \cdots \mathbf{S}_0(z), \quad \mathbf{D}_K \equiv \text{diag}(1/K, K), \quad \mathbf{S}_i \in \mathcal{U} \cup \mathcal{L}.$$

- Define the *gain scaling group*,  $\mathcal{D} \equiv \{\mathbf{D}_K : K \neq 0\}$ .

The *lifting cascade group* is  $\mathcal{C} \equiv \langle \mathcal{U} \cup \mathcal{L} \rangle < \mathcal{W}$ .

$\mathcal{D}$  acts on  $\mathcal{U}$ ,  $\mathcal{L}$ ,  $\mathcal{C}$  via inner automorphisms,  $\gamma_K \mathbf{A}(z) \equiv \mathbf{D}_K \mathbf{A}(z) \mathbf{D}_K^{-1}$ .

We say “ $\mathcal{D}$  normalizes  $\mathcal{C}$ ,” or “ $\mathcal{C}$  is  $\mathcal{D}$ -invariant.”

- The *scaled lifting group* is  $\mathcal{S} \equiv \langle \mathcal{D} \cup \mathcal{C} \rangle = \mathcal{D}\mathcal{C}$ .
- The WS Group Lifting Factorization Thm. can be restated:  
 $\mathcal{W} = \mathcal{D}\mathcal{C} = \mathcal{S}$ , the scaled lifting group.

# Lifting Factorization of HS Filter Banks (messier) [2]

- The class  $\mathfrak{H}$  of unimodular HS filter banks does *not* form a group.
- One can factor whole-sample *antisymmetric* (WA) lifting filters off of *unequal-length* HS filter banks, but not off of *equal-length* HS filter banks.

# Lifting Factorization of HS Filter Banks (messier) [2]

- The class  $\mathfrak{H}$  of unimodular HS filter banks does *not* form a group.
- One can factor whole-sample *antisymmetric* (WA) lifting filters off of *unequal-length* HS filter banks, but not off of *equal-length* HS filter banks.
- Let  $\mathcal{U}$  (resp.,  $\mathcal{L}$ ) be the group of upper- (lower-)triangular lifting matrices with off-diagonal lifting filters antisymmetric about 0. Define  $\mathcal{C} \equiv \langle \mathcal{U} \cup \mathcal{L} \rangle$ ; then  $\gamma : \mathcal{D} \rightarrow \text{Aut}(\mathcal{C})$ , and  $\mathcal{S} \equiv \langle \mathcal{D} \cup \mathcal{C} \rangle = \mathcal{D}\mathcal{C}$ .
- Let  $\mathfrak{B}$  be the set (it's not a group) of *concentric equal length* unimodular HS “base” filter banks, which are centered at  $-1/2$ .

# Lifting Factorization of HS Filter Banks (messier) [2]

- The class  $\mathfrak{H}$  of unimodular HS filter banks does *not* form a group.
- One can factor whole-sample *antisymmetric* (WA) lifting filters off of *unequal-length* HS filter banks, but not off of *equal-length* HS filter banks.
- Let  $\mathcal{U}$  (resp.,  $\mathcal{L}$ ) be the group of upper- (lower-)triangular lifting matrices with off-diagonal lifting filters antisymmetric about 0. Define  $\mathcal{C} \equiv \langle \mathcal{U} \cup \mathcal{L} \rangle$ ; then  $\gamma : \mathcal{D} \rightarrow \text{Aut}(\mathcal{C})$ , and  $\mathcal{S} \equiv \langle \mathcal{D} \cup \mathcal{C} \rangle = \mathcal{D}\mathcal{C}$ .
- Let  $\mathfrak{B}$  be the set (it's not a group) of *concentric equal length* unimodular HS “base” filter banks, which are centered at  $-1/2$ .
- **Theorem:** (HS Lifting Factorization)  $\mathbf{H}(z) \in \mathfrak{H}$  iff it factors as

$$\mathbf{H}(z) = \mathbf{D}_K \mathbf{S}_N(z) \cdots \mathbf{S}_0(z) \mathbf{B}(z), \quad \mathbf{D}_K \in \mathcal{D}, \quad \mathbf{S}_i \in \mathcal{U} \cup \mathcal{L}, \quad \mathbf{B} \in \mathfrak{B};$$

i.e.,

$$\mathfrak{H} = \mathcal{D}\mathcal{C}\mathfrak{B} = \mathcal{S}\mathfrak{B}.$$

$\mathcal{S}$  captures the group-theoretic aspects of lifting for HS filter banks.

# How Unique Are Lifting Factorizations?

- Elementary matrix decompositions are highly nonunique in general. What about lifting factorizations?

# How Unique Are Lifting Factorizations?

- Elementary matrix decompositions are highly nonunique in general. What about lifting factorizations?
- Some nonuniqueness issues are trivial:  
A lifting cascade is called *irreducible* if the lifting matrices strictly alternate between upper- and lower-triangular.

# How Unique Are Lifting Factorizations?

- Elementary matrix decompositions are highly nonunique in general. What about lifting factorizations?
- Some nonuniqueness issues are trivial:  
A lifting cascade is called *irreducible* if the lifting matrices strictly alternate between upper- and lower-triangular.
- Positing irreducibility is far from sufficient to ensure unique lifting factorizations:

$$\begin{bmatrix} 1 & 0 \\ 0 & 1 \end{bmatrix} = \begin{bmatrix} 1 & -2 \\ 0 & 1 \end{bmatrix} \begin{bmatrix} 1 & 0 \\ -1/2 & 1 \end{bmatrix} \begin{bmatrix} 1 & 1 \\ 0 & 1 \end{bmatrix} \begin{bmatrix} 1 & 0 \\ 1 & 1 \end{bmatrix} \cdot \\ \begin{bmatrix} 1 & 1/4 \\ 0 & 1 \end{bmatrix} \begin{bmatrix} 1 & 0 \\ -2 & 1 \end{bmatrix} \begin{bmatrix} 1 & -1/2 \\ 0 & 1 \end{bmatrix} \begin{bmatrix} 1 & 0 \\ 1 & 1 \end{bmatrix}$$

# Equivalence Modulo Rescaling

- Consider the Haar filter bank,  $B_0(z) = (z + 1)/2$ ,  $B_1(z) = z - 1$ :

$$\begin{aligned}\mathbf{B}_{haar}(z) &\equiv \begin{bmatrix} 1/2 & 1/2 \\ -1 & 1 \end{bmatrix} = \begin{bmatrix} 1 & 1/2 \\ 0 & 1 \end{bmatrix} \begin{bmatrix} 1 & 0 \\ -1 & 1 \end{bmatrix} \\ &= \begin{bmatrix} 1/2 & 0 \\ 0 & 2 \end{bmatrix} \begin{bmatrix} 1 & 0 \\ -1/2 & 1 \end{bmatrix} \begin{bmatrix} 1 & 1 \\ 0 & 1 \end{bmatrix} \equiv \mathbf{D}_2 \mathbf{B}'_{haar}(z).\end{aligned}$$

# Equivalence Modulo Rescaling

- Consider the Haar filter bank,  $B_0(z) = (z + 1)/2$ ,  $B_1(z) = z - 1$ :

$$\begin{aligned}\mathbf{B}_{haar}(z) &\equiv \begin{bmatrix} 1/2 & 1/2 \\ -1 & 1 \end{bmatrix} = \begin{bmatrix} 1 & 1/2 \\ 0 & 1 \end{bmatrix} \begin{bmatrix} 1 & 0 \\ -1 & 1 \end{bmatrix} \\ &= \begin{bmatrix} 1/2 & 0 \\ 0 & 2 \end{bmatrix} \begin{bmatrix} 1 & 0 \\ -1/2 & 1 \end{bmatrix} \begin{bmatrix} 1 & 1 \\ 0 & 1 \end{bmatrix} \equiv \mathbf{D}_2 \mathbf{B}'_{haar}(z).\end{aligned}$$

- Nonunique factorizations can propagate via lifting. E.g., if

$$\mathbf{H}(z) = \mathbf{S}_N(z) \cdots \mathbf{S}_1(z) \mathbf{S}_0(z) \mathbf{B}_{haar}(z)$$

then, using  $\mathbf{B}'_{haar}(z)$  and the group action of  $\mathcal{D}$  on  $\mathcal{C}$ ,

$$\mathbf{H}(z) = \mathbf{D}_2 \mathbf{S}'_N(z) \cdots \mathbf{S}'_1(z) \mathbf{S}'_0(z) \mathbf{B}'_{haar}(z)$$

where  $\mathbf{S}_i(z) = \gamma_2 \mathbf{S}'_i(z)$ .

# Equivalence Modulo Rescaling

- Consider the Haar filter bank,  $B_0(z) = (z + 1)/2$ ,  $B_1(z) = z - 1$ :

$$\begin{aligned}\mathbf{B}_{haar}(z) &\equiv \begin{bmatrix} 1/2 & 1/2 \\ -1 & 1 \end{bmatrix} = \begin{bmatrix} 1 & 1/2 \\ 0 & 1 \end{bmatrix} \begin{bmatrix} 1 & 0 \\ -1 & 1 \end{bmatrix} \\ &= \begin{bmatrix} 1/2 & 0 \\ 0 & 2 \end{bmatrix} \begin{bmatrix} 1 & 0 \\ -1/2 & 1 \end{bmatrix} \begin{bmatrix} 1 & 1 \\ 0 & 1 \end{bmatrix} \equiv \mathbf{D}_2 \mathbf{B}'_{haar}(z).\end{aligned}$$

- Nonunique factorizations can propagate via lifting. E.g., if

$$\mathbf{H}(z) = \mathbf{S}_N(z) \cdots \mathbf{S}_1(z) \mathbf{S}_0(z) \mathbf{B}_{haar}(z)$$

then, using  $\mathbf{B}'_{haar}(z)$  and the group action of  $\mathcal{D}$  on  $\mathcal{C}$ ,

$$\mathbf{H}(z) = \mathbf{D}_2 \mathbf{S}'_N(z) \cdots \mathbf{S}'_1(z) \mathbf{S}'_0(z) \mathbf{B}'_{haar}(z)$$

where  $\mathbf{S}_i(z) = \gamma_2 \mathbf{S}'_i(z)$ .

- Two lifting factorizations that differ in this manner are said to be *equivalent modulo rescaling*.

# Group Lifting Structures [3]

- Does avoiding constant lifting filters help (cf. Haar)? Nope:

$$\mathbf{I} = \begin{bmatrix} 1 & (-z^2/4)(1 - z^{-1}) \\ 0 & 1 \end{bmatrix} \begin{bmatrix} 1 & 0 \\ -4(1 + z^{-1}) & 1 \end{bmatrix} \begin{bmatrix} 1 & (5/4)(1 - z^{-1}) \\ 0 & 1 \end{bmatrix} \\ \cdot \begin{bmatrix} 1 & 0 \\ -(1 + z^{-1}) & 1 \end{bmatrix} \begin{bmatrix} 1 & -z^2(1 - z^{-1}) \\ 0 & 1 \end{bmatrix} \begin{bmatrix} 1 & 0 \\ 5z^{-2}(1 + z^{-1}) & 1 \end{bmatrix}$$

# Group Lifting Structures [3]

- Does avoiding constant lifting filters help (cf. Haar)? Nope:

$$\mathbf{I} = \begin{bmatrix} 1 & (-z^2/4)(1 - z^{-1}) \\ 0 & 1 \end{bmatrix} \begin{bmatrix} 1 & 0 \\ -4(1 + z^{-1}) & 1 \end{bmatrix} \begin{bmatrix} 1 & (5/4)(1 - z^{-1}) \\ 0 & 1 \end{bmatrix} \\ \cdot \begin{bmatrix} 1 & 0 \\ -(1 + z^{-1}) & 1 \end{bmatrix} \begin{bmatrix} 1 & -z^2(1 - z^{-1}) \\ 0 & 1 \end{bmatrix} \begin{bmatrix} 1 & 0 \\ 5z^{-2}(1 + z^{-1}) & 1 \end{bmatrix}$$

- The Laurent orders of the partial products in this cascade increase (up to 4) but then *decrease* back to 0. This suggests preventing such pathologies by restricting the universe of “admissible” lifting matrices. This requires machinery.

# Group Lifting Structures [3]

- Does avoiding constant lifting filters help (cf. Haar)? Nope:

$$\mathbf{I} = \begin{bmatrix} 1 & (-z^2/4)(1 - z^{-1}) \\ 0 & 1 \end{bmatrix} \begin{bmatrix} 1 & 0 \\ -4(1 + z^{-1}) & 1 \end{bmatrix} \begin{bmatrix} 1 & (5/4)(1 - z^{-1}) \\ 0 & 1 \end{bmatrix} \\ \cdot \begin{bmatrix} 1 & 0 \\ -(1 + z^{-1}) & 1 \end{bmatrix} \begin{bmatrix} 1 & -z^2(1 - z^{-1}) \\ 0 & 1 \end{bmatrix} \begin{bmatrix} 1 & 0 \\ 5z^{-2}(1 + z^{-1}) & 1 \end{bmatrix}$$

- The Laurent orders of the partial products in this cascade increase (up to 4) but then *decrease* back to 0. This suggests preventing such pathologies by restricting the universe of “admissible” lifting matrices. This requires machinery.
- A *group lifting structure* is an ordered 4-tuple,  $\mathfrak{S} \equiv (\mathcal{D}, \mathcal{U}, \mathcal{L}, \mathfrak{B})$ , where  $\mathcal{D}$  is a gain scaling group,  $\mathcal{U}$  and  $\mathcal{L}$  are upper- and lower-triangular lifting matrix groups, and  $\mathfrak{B}$  is a set of base filter banks. As before,  $\mathcal{C} \equiv \langle \mathcal{U} \cup \mathcal{L} \rangle$  and  $\mathcal{S} \equiv \langle \mathcal{D} \cup \mathcal{C} \rangle$ .  
The universe of all filter banks generated by  $\mathfrak{S}$  is  $\mathcal{DCB}$ .

# Linear Phase Group Lifting Structures

- The group lifting structure,  $\mathfrak{G}_W$ , for WS filter banks is:

$$\mathcal{D} = \{\mathbf{D}_K : K \neq 0\}$$

$$\mathcal{U} = \{\text{upper triangular } \mathbf{S}(z) : S(z^{-1}) = z\mathbf{S}(z)\}$$

$$\mathcal{L} = \{\text{lower triangular } \mathbf{S}(z) : S(z^{-1}) = z^{-1}\mathbf{S}(z)\}$$

$$\mathfrak{B} = \{\mathbf{I}\}.$$

# Linear Phase Group Lifting Structures

- The group lifting structure,  $\mathfrak{G}_W$ , for WS filter banks is:

$$\mathcal{D} = \{\mathbf{D}_K : K \neq 0\}$$

$$\mathcal{U} = \{\text{upper triangular } \mathbf{S}(z) : S(z^{-1}) = zS(z)\}$$

$$\mathcal{L} = \{\text{lower triangular } \mathbf{S}(z) : S(z^{-1}) = z^{-1}S(z)\}$$

$$\mathfrak{B} = \{\mathbf{I}\}.$$

- The group lifting structure,  $\mathfrak{G}_H$ , for HS filter banks is:

$$\mathcal{D} = \{\mathbf{D}_K : K \neq 0\}$$

$$\mathcal{U} = \{\text{upper triangular } \mathbf{S}(z) : S(z^{-1}) = -S(z)\}$$

$$\mathcal{L} = \{\text{lower triangular } \mathbf{S}(z) : S(z^{-1}) = -S(z)\}$$

$$\mathfrak{B} = \{\text{concentric equal-length HS filter banks}\}$$

# Unique Group Lifting Factorization Theorem [3]

- $\mathcal{G}$  is a  $\mathcal{D}$ -invariant group lifting structure if  $\mathcal{U}$ ,  $\mathcal{L}$ ,  $\mathcal{C}$  are  $\mathcal{D}$ -invariant.

# Unique Group Lifting Factorization Theorem [3]

- $\mathcal{G}$  is a  $\mathcal{D}$ -invariant group lifting structure if  $\mathcal{U}$ ,  $\mathcal{L}$ ,  $\mathcal{C}$  are  $\mathcal{D}$ -invariant.
- $\mathcal{G}$  is *strictly polyphase order-increasing* if, for every irreducible lifting cascade  $\mathbf{S}_N(z) \cdots \mathbf{S}_0(z) \mathbf{B}(z) \in \mathcal{CB}$ , we have

$$\text{order}(\mathbf{S}_k(z) \cdots \mathbf{S}_0(z) \mathbf{B}(z)) > \text{order}(\mathbf{S}_{k-1}(z) \cdots \mathbf{B}(z)) , \quad k \leq N.$$

# Unique Group Lifting Factorization Theorem [3]

- $\mathfrak{G}$  is a  $\mathcal{D}$ -invariant group lifting structure if  $\mathcal{U}$ ,  $\mathcal{L}$ ,  $\mathcal{C}$  are  $\mathcal{D}$ -invariant.
- $\mathfrak{G}$  is *strictly polyphase order-increasing* if, for every irreducible lifting cascade  $\mathbf{S}_N(z) \cdots \mathbf{S}_0(z) \mathbf{B}(z) \in \mathcal{C}\mathfrak{B}$ , we have

$$\text{order}(\mathbf{S}_k(z) \cdots \mathbf{S}_0(z) \mathbf{B}(z)) > \text{order}(\mathbf{S}_{k-1}(z) \cdots \mathbf{B}(z)) , \quad k \leq N.$$

- **Theorem:** Let  $\mathfrak{G} = (\mathcal{D}, \mathcal{U}, \mathcal{L}, \mathfrak{B})$  be  $\mathcal{D}$ -invariant and strictly polyphase order-increasing. Suppose  $\mathbf{H}(z)$  has two irreducible lifting factorizations in  $\mathcal{D}\mathcal{C}\mathfrak{B}$ :

$$\begin{aligned} \mathbf{H}(z) &= \mathbf{D}_K \mathbf{S}_{N-1}(z) \cdots \mathbf{S}_0(z) \mathbf{B}(z) \\ &= \mathbf{D}_{K'} \mathbf{S}'_{N'-1}(z) \cdots \mathbf{S}'_0(z) \mathbf{B}'(z) . \end{aligned}$$

Then the factorizations are equivalent modulo rescaling:  $N' = N$ ,

$$\mathbf{B}'(z) = \mathbf{D}_\alpha \mathbf{B}(z), \quad \alpha \equiv K/K', \quad \text{and} \quad \mathbf{S}'_i(z) = \gamma_\alpha \mathbf{S}_i(z) \text{ for } i < N.$$

If, e.g.,  $\mathfrak{B} = \{\mathbf{I}\}$  then factorizations are necessarily *unique*.

# Uniqueness of Linear Phase Lifting Factorizations [4]

- After many tedious calculations needed to verify the polyphase order-increasing property, we get

**Theorem:** Every filter bank in  $\mathcal{W}$  has a unique irreducible group lifting factorization in  $\mathfrak{S}_{\mathcal{W}}$ .

**Application:** WS filter banks can be specified (via linear phase lifting) in JPEG 2000 Part 2 Annex G in one and only one way.

# Uniqueness of Linear Phase Lifting Factorizations [4]

- After many tedious calculations needed to verify the polyphase order-increasing property, we get

**Theorem:** Every filter bank in  $\mathcal{W}$  has a unique irreducible group lifting factorization in  $\mathfrak{S}_{\mathcal{W}}$ .

**Application:** WS filter banks can be specified (via linear phase lifting) in JPEG 2000 Part 2 Annex G in one and only one way.

- Similarly, after more tedious calculations,

**Theorem:** Every filter bank in  $\mathfrak{H}$  has an irreducible group lifting factorization in  $\mathfrak{S}_{\mathfrak{H}}$  that is unique modulo rescaling.

# Uniqueness of Linear Phase Lifting Factorizations [4]

- After many tedious calculations needed to verify the polyphase order-increasing property, we get

**Theorem:** Every filter bank in  $\mathcal{W}$  has a unique irreducible group lifting factorization in  $\mathfrak{S}_{\mathcal{W}}$ .

**Application:** WS filter banks can be specified (via linear phase lifting) in JPEG 2000 Part 2 Annex G in one and only one way.

- Similarly, after more tedious calculations,

**Theorem:** Every filter bank in  $\mathfrak{H}$  has an irreducible group lifting factorization in  $\mathfrak{S}_{\mathfrak{H}}$  that is unique modulo rescaling.

- **Application:** We now apply these unique factorization results to determine the group-theoretic structure of the WS and HS lifting cascade groups,  $\mathcal{C}$ , and scaled lifting groups,  $\mathcal{S}$ , up to isomorphism.

# Free Product Structure of Lifting Cascade Groups [5]

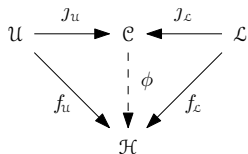

Uniqueness of group lifting factorizations implies that  $\mathcal{C}$  satisfies the universal mapping (categorical) characterization of free products. Let  $j_{\mathcal{U}}$  and  $j_{\mathcal{L}}$  be the inclusions of  $\mathcal{U}$  and  $\mathcal{L}$  into  $\mathcal{C}$ . Then  $\mathcal{C}$  is the *free product* of  $\mathcal{U}$  and  $\mathcal{L}$  if, for any group  $\mathcal{H}$  and homomorphisms  $f_{\mathcal{U}}, f_{\mathcal{L}}$  there exists a unique homomorphism  $\phi : \mathcal{C} \rightarrow \mathcal{H}$  such that the diagram commutes.

# Free Product Structure of Lifting Cascade Groups [5]

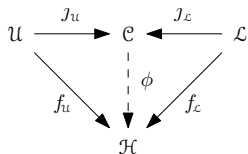

Uniqueness of group lifting factorizations implies that  $\mathcal{C}$  satisfies the universal mapping (categorical) characterization of free products. Let  $j_{\mathcal{U}}$  and  $j_{\mathcal{L}}$  be the inclusions of  $\mathcal{U}$  and  $\mathcal{L}$  into  $\mathcal{C}$ . Then  $\mathcal{C}$  is the *free product* of  $\mathcal{U}$  and  $\mathcal{L}$  if, for any group  $\mathcal{H}$  and homomorphisms  $f_{\mathcal{U}}, f_{\mathcal{L}}$  there exists a unique homomorphism  $\phi : \mathcal{C} \rightarrow \mathcal{H}$  such that the diagram commutes.

- There is a canonical “reduced word construction” of free products, which we denote  $\mathcal{U} * \mathcal{L}$ . The intuition is that unique factorization puts irreducible group lifting factorizations in 1-1 correspondence with canonical reduced words on  $\mathcal{U} \cup \mathcal{L}$ .

# Free Product Structure of Lifting Cascade Groups [5]

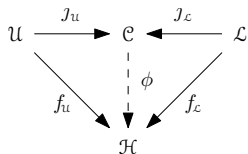

Uniqueness of group lifting factorizations implies that  $\mathcal{C}$  satisfies the universal mapping (categorical) characterization of free products. Let  $j_{\mathcal{U}}$  and  $j_{\mathcal{L}}$  be the inclusions of  $\mathcal{U}$  and  $\mathcal{L}$  into  $\mathcal{C}$ . Then  $\mathcal{C}$  is the *free product* of  $\mathcal{U}$  and  $\mathcal{L}$  if, for any group  $\mathcal{H}$  and homomorphisms  $f_{\mathcal{U}}, f_{\mathcal{L}}$  there exists a unique homomorphism  $\phi : \mathcal{C} \rightarrow \mathcal{H}$  such that the diagram commutes.

- There is a canonical “reduced word construction” of free products, which we denote  $\mathcal{U} * \mathcal{L}$ . The intuition is that unique factorization puts irreducible group lifting factorizations in 1-1 correspondence with canonical reduced words on  $\mathcal{U} \cup \mathcal{L}$ .
- **Theorem:** Let  $\mathcal{U}$  and  $\mathcal{L}$  be upper- and lower-triangular lifting matrix groups with lifting cascade group  $\mathcal{C} \equiv \langle \mathcal{U} \cup \mathcal{L} \rangle$ . If every element of  $\mathcal{C}$  has a unique irreducible group lifting factorization over  $\mathcal{U} \cup \mathcal{L}$  then  $\mathcal{C}$  is isomorphic to the free product of  $\mathcal{U}$  and  $\mathcal{L}$ :

$$\rho: \mathcal{C} \xrightarrow{\cong} \mathcal{U} * \mathcal{L}.$$

# Scaled Lifting Groups Are Semidirect Products [5]

The *hypotheses* of the Unique Factorization Theorem also provide the group-theoretic structure of  $\mathcal{S}$ , without explicitly using uniqueness.

- $\mathcal{G} = \langle \mathcal{K} \cup \mathcal{Q} \rangle$  is an (*internal*) *semidirect product of  $\mathcal{K}$  by  $\mathcal{Q}$* , denoted  $\mathcal{G} = \mathcal{Q} \ltimes \mathcal{K}$ , if the following axioms are satisfied.

$$\mathcal{K} \triangleleft \mathcal{G} \quad (\mathcal{K} \text{ is a normal subgroup of } \mathcal{G}) \quad (1)$$

$$\mathcal{K} \cap \mathcal{Q} = 1_{\mathcal{G}} \quad (\text{the trivial group}) \quad (2)$$

# Scaled Lifting Groups Are Semidirect Products [5]

The *hypotheses* of the Unique Factorization Theorem also provide the group-theoretic structure of  $\mathcal{S}$ , without explicitly using uniqueness.

- $\mathcal{G} = \langle \mathcal{K} \cup \mathcal{Q} \rangle$  is an (*internal*) *semidirect product of  $\mathcal{K}$  by  $\mathcal{Q}$* , denoted  $\mathcal{G} = \mathcal{Q} \ltimes \mathcal{K}$ , if the following axioms are satisfied.

$$\mathcal{K} \triangleleft \mathcal{G} \quad (\mathcal{K} \text{ is a normal subgroup of } \mathcal{G}) \quad (1)$$

$$\mathcal{K} \cap \mathcal{Q} = 1_{\mathcal{G}} \quad (\text{the trivial group}) \quad (2)$$

- **Theorem:** If  $\mathcal{G}$  is a  $\mathcal{D}$ -invariant, order-increasing group lifting structure then  $\mathcal{S}$  is the semidirect product of  $\mathcal{C}$  by  $\mathcal{D}$ :  $\mathcal{S} = \mathcal{D} \ltimes \mathcal{C}$ .  
**Idea:** Axiom (1) follows from  $\mathcal{D}$ -invariance, axiom (2) from the order-increasing hypothesis, without invoking unique factorization.

# Scaled Lifting Groups Are Semidirect Products [5]

The *hypotheses* of the Unique Factorization Theorem also provide the group-theoretic structure of  $\mathcal{S}$ , without explicitly using uniqueness.

- $\mathcal{G} = \langle \mathcal{K} \cup \mathcal{Q} \rangle$  is an (*internal*) *semidirect product of  $\mathcal{K}$  by  $\mathcal{Q}$* , denoted  $\mathcal{G} = \mathcal{Q} \ltimes \mathcal{K}$ , if the following axioms are satisfied.

$$\mathcal{K} \triangleleft \mathcal{G} \quad (\mathcal{K} \text{ is a normal subgroup of } \mathcal{G}) \quad (1)$$

$$\mathcal{K} \cap \mathcal{Q} = 1_{\mathcal{G}} \quad (\text{the trivial group}) \quad (2)$$

- **Theorem:** If  $\mathcal{G}$  is a  $\mathcal{D}$ -invariant, order-increasing group lifting structure then  $\mathcal{S}$  is the semidirect product of  $\mathcal{C}$  by  $\mathcal{D}$ :  $\mathcal{S} = \mathcal{D} \ltimes \mathcal{C}$ .  
**Idea:** Axiom (1) follows from  $\mathcal{D}$ -invariance, axiom (2) from the order-increasing hypothesis, without invoking unique factorization.
- **Corollary:** Combining both theorems, if  $\mathcal{G}$  is a  $\mathcal{D}$ -invariant, order-increasing group lifting structure then

$$\mathcal{S} \cong \mathcal{D} \ltimes_{\theta} (\mathcal{U} * \mathcal{L}), \quad \text{where} \quad \theta_k \equiv \rho \circ \gamma_k \circ \rho^{-1}.$$

This gives the structure of the WS group,  $\mathcal{W} = \mathcal{S}_{\mathcal{W}} \cong \mathcal{D} \ltimes_{\theta} (\mathcal{U} * \mathcal{L})$ .

# Analogy with “Nonabelian Vector Spaces” [5]

To what extent are scaled lifting groups “nonabelian vector spaces”?  
Find analogues for the vector space axioms when vector add. is replaced by matrix mult. and scalar mult. by scaling automorphisms.

$$1_{\mathbb{F}} \mathbf{v} = \mathbf{v} \quad (3)$$

$$a(b\mathbf{v}) = (ab)\mathbf{v} \quad (4)$$

$$a(\mathbf{u} + \mathbf{v}) = a\mathbf{u} + a\mathbf{v} \quad (5)$$

$$(a + b)\mathbf{v} = a\mathbf{v} + b\mathbf{v} \quad (6)$$

# Analogy with “Nonabelian Vector Spaces” [5]

To what extent are scaled lifting groups “nonabelian vector spaces”?  
Find analogues for the vector space axioms when vector add. is replaced by matrix mult. and scalar mult. by scaling automorphisms.

$$1_{\mathbb{F}} \mathbf{v} = \mathbf{v} \quad (3)$$

$$a(b\mathbf{v}) = (ab)\mathbf{v} \quad (4)$$

$$a(\mathbf{u} + \mathbf{v}) = a\mathbf{u} + a\mathbf{v} \quad (5)$$

$$(a + b)\mathbf{v} = a\mathbf{v} + b\mathbf{v} \quad (6)$$

- (3) becomes  $\gamma_1 \mathbf{E} = \mathbf{E}$ , which is trivially true.

# Analogy with “Nonabelian Vector Spaces” [5]

To what extent are scaled lifting groups “nonabelian vector spaces”?  
Find analogues for the vector space axioms when vector add. is replaced by matrix mult. and scalar mult. by scaling automorphisms.

$$1_{\mathbb{F}} \mathbf{v} = \mathbf{v} \quad (3)$$

$$a(b\mathbf{v}) = (ab)\mathbf{v} \quad (4)$$

$$a(\mathbf{u} + \mathbf{v}) = a\mathbf{u} + a\mathbf{v} \quad (5)$$

$$(a + b)\mathbf{v} = a\mathbf{v} + b\mathbf{v} \quad (6)$$

- (3) becomes  $\gamma_1 \mathbf{E} = \mathbf{E}$ , which is trivially true.
- (4) becomes  $\gamma_{k'}(\gamma_k \mathbf{E}) = \gamma_{k'k} \mathbf{E}$ , which is the group action of  $\mathcal{D}$ .

# Analogy with “Nonabelian Vector Spaces” [5]

To what extent are scaled lifting groups “nonabelian vector spaces”?  
Find analogues for the vector space axioms when vector add. is replaced by matrix mult. and scalar mult. by scaling automorphisms.

$$1_{\mathbb{F}} \mathbf{v} = \mathbf{v} \quad (3)$$

$$a(b\mathbf{v}) = (ab)\mathbf{v} \quad (4)$$

$$a(\mathbf{u} + \mathbf{v}) = a\mathbf{u} + a\mathbf{v} \quad (5)$$

$$(a + b)\mathbf{v} = a\mathbf{v} + b\mathbf{v} \quad (6)$$

- (3) becomes  $\gamma_1 \mathbf{E} = \mathbf{E}$ , which is trivially true.
- (4) becomes  $\gamma_{k'}(\gamma_k \mathbf{E}) = \gamma_{k'k} \mathbf{E}$ , which is the group action of  $\mathcal{D}$ .
- (5) becomes  $\gamma_k(\mathbf{E}\mathbf{F}) = (\gamma_k \mathbf{E})(\gamma_k \mathbf{F})$ , which holds for automorphisms.

# Analogy with “Nonabelian Vector Spaces” [5]

To what extent are scaled lifting groups “nonabelian vector spaces”? Find analogues for the vector space axioms when vector add. is replaced by matrix mult. and scalar mult. by scaling automorphisms.

$$1_{\mathbb{F}} \mathbf{v} = \mathbf{v} \quad (3)$$

$$a(b\mathbf{v}) = (ab)\mathbf{v} \quad (4)$$

$$a(\mathbf{u} + \mathbf{v}) = a\mathbf{u} + a\mathbf{v} \quad (5)$$

$$(a + b)\mathbf{v} = a\mathbf{v} + b\mathbf{v} \quad (6)$$

- (3) becomes  $\gamma_1 \mathbf{E} = \mathbf{E}$ , which is trivially true.
- (4) becomes  $\gamma_{k'}(\gamma_k \mathbf{E}) = \gamma_{k'k} \mathbf{E}$ , which is the group action of  $\mathcal{D}$ .
- (5) becomes  $\gamma_k(\mathbf{E}\mathbf{F}) = (\gamma_k \mathbf{E})(\gamma_k \mathbf{F})$ , which holds for automorphisms.
- (6) is problematic since automorphisms don't always have additive structure. Suppose  $\mathcal{D} \equiv \{\mathbf{D}_K : K > 0\}$ ; then the analog of (6) is

$$\gamma_{k+k'} \mathbf{E} = (\gamma_k \mathbf{E})(\gamma_{k'} \mathbf{E}). \quad (7)$$

(cf. the matrix exponential function)

# “Nonabelian Vector Spaces” cont. [5]

Property (7) is not satisfied by  $\gamma$ , but does it hold for *any* (redefined) automorphic group action? **NO:**

# “Nonabelian Vector Spaces” cont. [5]

Property (7) is not satisfied by  $\gamma$ , but does it hold for *any* (redefined) automorphic group action? **NO:**

- **Theorem:** Let  $\mathcal{R} \subset \mathbb{F}$  be a multiplicative group that's closed under addition. If there exists an automorphic group action  $\gamma: \mathcal{R} \rightarrow \text{Aut}(\mathcal{S})$  that also satisfies (7) then  $\mathcal{S}$  is abelian.

# “Nonabelian Vector Spaces” cont. [5]

Property (7) is not satisfied by  $\gamma$ , but does it hold for *any* (redefined) automorphic group action? **NO:**

- **Theorem:** Let  $\mathcal{R} \subset \mathbb{F}$  be a multiplicative group that's closed under addition. If there exists an automorphic group action  $\gamma: \mathcal{R} \rightarrow \text{Aut}(\mathcal{S})$  that also satisfies (7) then  $\mathcal{S}$  is abelian.
- **Interpretation:** No such thing as a “nonabelian module.”
- While they have many of the properties of vector spaces, these scaled lifting groups should perhaps be viewed instead as infinite-dimensional (non-nilpotent) generalizations of the *homogeneous groups* introduced by Folland and Stein, generalizing the Heisenberg group.

- Simplify the unique factorization arguments in [3, 4].
- Develop a *causal* version of the group-theoretic approach with state-space implications.
- Numerical filter bank implementations and design applications.
- Complete the structure theory for HS filter banks.

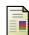

C. M. Brislawn, “On the group-theoretic structure of lifted filter banks,” in *Excursions in Harmonic Analysis, Vol. 2*, ser. Applied and Numerical Harmonic Analysis, T. Andrews, R. Balan, J. Benedetto, W. Czaja, and K. Okoudjou, Eds. Boston: Birkhäuser, 2013, pp. 113–135, invited book chapter.  
[http://dx.doi.org/10.1007/978-0-8176-8379-5\\_6](http://dx.doi.org/10.1007/978-0-8176-8379-5_6). [Online]. Available: <http://arxiv.org/abs/1310.0530>

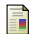

C. M. Brislawn and B. Wohlberg, “The polyphase-with-advance representation and linear phase lifting factorizations,” *IEEE Trans. Signal Process.*, vol. 54, no. 6, pp. 2022–2034, Jun. 2006. [Online]. Available: <http://dx.doi.org/10.1109/TSP.2006.872582>

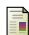

C. M. Brislawn, “Group lifting structures for multirate filter banks I: Uniqueness of lifting factorizations,” *IEEE Trans. Signal Process.*, vol. 58, no. 4, pp. 2068–2077, Apr. 2010,  
<http://dx.doi.org/10.1109/TSP.2009.2039816>. [Online]. Available: <http://arxiv.org/abs/1310.2206>

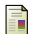

——, “Group lifting structures for multirate filter banks II: Linear phase filter banks,” *IEEE Trans. Signal Process.*, vol. 58, no. 4, pp. 2078–2087, Apr. 2010,  
<http://dx.doi.org/10.1109/TSP.2009.2039818>. [Online]. Available:  
<http://arxiv.org/abs/1310.2208>

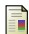

——, “Group-theoretic structure of linear phase multirate filter banks,” *IEEE Trans. Information Theory*, vol. 59, no. 9, pp. 5842–5859, Sept. 2013,  
<http://dx.doi.org/10.1109/TIT.2013.2259292>. [Online]. Available:  
<http://arxiv.org/abs/1309.7665>
